# Supplementary material for: OpenSU3D: Open World 3D Scene Understanding using Foundation Models
Source: arXiv:2407.14279 source file (2024-09-15)
Supplement: Supplementary file 1 [file model.tex]

\begin{figure}[h]
  \centering
  \modelclip{1}{double sofa}
  \modelclip{2}{single sofa}
\caption{\textbf{Text-Instance Similarity Heatmaps.} For a text query, per-instance cosine similarity heatmaps for different CLIP models. \textcolor{red!50!black}{\ensuremath{\blacksquare}}: max, \textcolor{blue!20!black}{\ensuremath{\blacksquare}}: min similarity.}
\vspace{-0.5cm} % Adjust this value to reduce the gap
  \label{fig:clip_compare}
\end{figure}
